# Supplementary material for: Double-loop hysteresis of multisite dilute Sr(Y$_{1-x}$Dy$_x$)$_2$O$_4$ single crystal Kramers paramagnets: electron-phonon interaction, quantum tunneling and cross-relaxation
Source: arXiv:2310.18947 source file (2023-10-29)
Supplement: Supplementary file 1 [file Supplementary_Material_Malkin_etal_SrY2O4_Dy_Hysteresis_2023.pdf]

Supplemental Material

# Double-loop hysteresis of multisite dilute $Sr(Y_{1-x}Dy_x)_2O_4$ single crystal Kramers paramagnets: electron-phonon interaction, quantum tunneling and cross-relaxation

B. Z. Malkin[1], R. V. Yusupov[1], I. F. Gilmutdinov[1], R. G. Batulin[1], A. G. Kiiamov[1], B. F. Gabbasov[1], S. I. Nikitin[1], and B. Barbara[2]

[1] Institute of Physics, Kazan Federal University, 420008 Kazan, Russian Federation

[2] Institut Néel, CNRS/UGA UPR2940 and Université Grenoble-Alpes, 25 Avenue des Martyrs BP 166, 38042 Grenoble Cedex 9, France

## Samples

Single crystalline samples of $SrY_2O_4$ compound doped with rare-earth $Dy^{3+}$ ions were grown by the optical floating zone technique in an air atmosphere under ambient pressure from a ceramic feed to a polycrystalline seed [S1,S2]. Crystal growth was carried out with the FZ-T-4000-H-VII-VPO-PC setup equipped with four 1-kW halogen lamps (Crystal Systems Corp., Japan). The growth rate was 4 mm/hour. Both the seed and the feed were obtained by firing a rod that had been compacted under 150 bar hydrostatic pressure at 1400°C. The $Sr(Y_{1-x}Dy_x)_2O_4$ powders used as a material for a rod was synthesized by the high-temperature solid-state reaction from the stoichiometric mixture of $SrCO_3$ and $Y_2O_3$, with a partial substitution of $Y_2O_3$ for $Dy_2O_3$. The samples with two doping values were synthesized and grown, $x = 0.0001$ and $x = 0.005$. The purity of the initial components was not worse than 99.95% (Alfa Aesar). The single phase composition of the synthesized powder was verified by the powder X-ray diffraction (Bruker D8 Advance). The symmetry of the crystal structure of $SrY_2O_4$ compound is orthorhombic, space group *Pnam* (No. 62, $D_{2h}^{16}$) [S3]. Single-crystal samples were oriented with the same Bruker D8 Advance diffractometer with the use of the Euler craddle. Orientation accuracy was $\pm 2$ degrees. The samples had a shape of a 2-3 mm size rectangular parallelepiped with the faces perpendicular to the crystallographic *a*, *b* and *c* axes.

## Physical characteristics of dysprosium isotopes [S4]

Natural abundance $C_{na}$, nuclear spin *I*, gyromagnetic ratio $\gamma$, nuclear quadrupole moment *Q* are presented below. The total content of even isotopes equals $C_{nae}$ = 56.2 %, in particular, $C_{na}$ ($^{162}$Dy) = 25.5 %, $C_{na}$ ($^{164}$Dy) = 28.3 %. For odd isotopes,

$C_{na}$ ($^{161}$Dy) = 18.9 %, $I = 5/2$, $\gamma$ = –1.465 MHz/T, $Q = 2.36 \cdot 10^{-28}$ m$^2$,

$C_{na}$ ($^{163}$Dy) = 24.9 %, $I = 5/2$, $\gamma$ = 2.03 MHz/T, $Q = 2.46 \cdot 10^{-28}$ m$^2$.

## Structural parameters of $SrY_2O_4$

Fragments of quasi-one-dimensional structure of $SrY_2O_4$ crystal lattice are shown in Fig. S1.

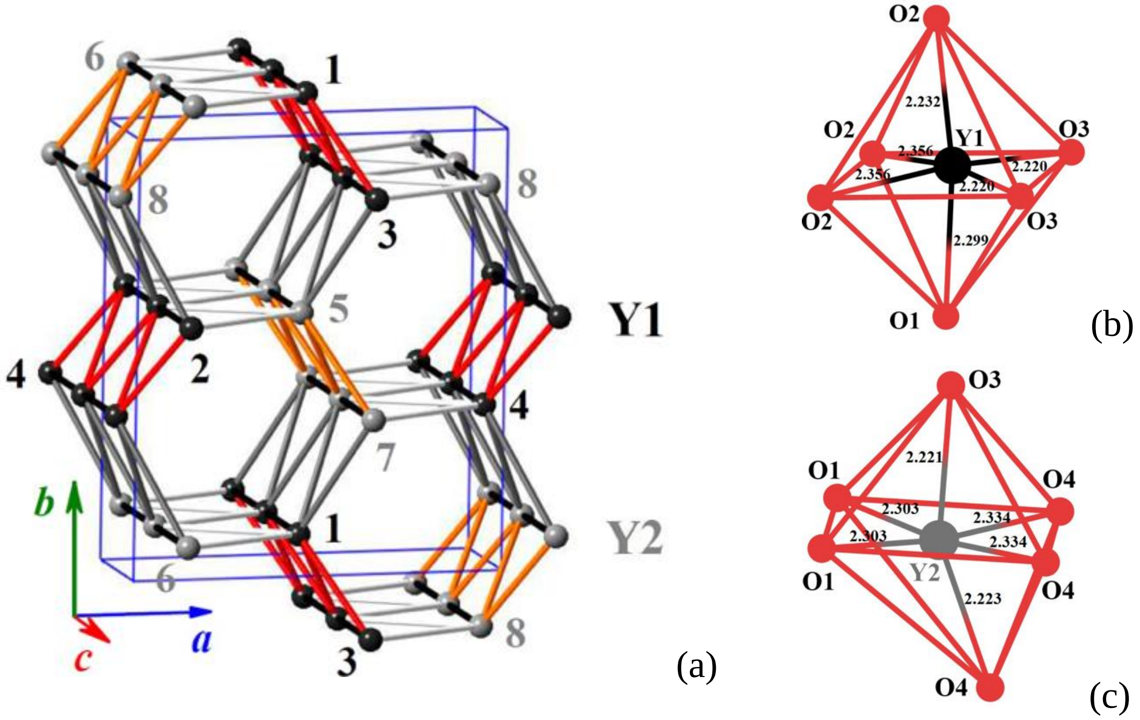


**Fig. S1**. (a) Yttrium sublattices in $SrY_2O_4$ crystal lattice, (b,c) the nearest oxygen surroundings of Y1 and Y2 sites.

The unit cell contains 4 formula units. Eight $Y^{3+}$ ions at the Wyckoff positions 4*c* form two subsystems Y1 and Y2, each subsystem contains 4 equivalent sublattices with the radius-vectors $\boldsymbol{r}_{n,\lambda}$ of $Y^{3+}$ ions, $\boldsymbol{r}_{1,\lambda} = [ax_\lambda, by_\lambda, 0.25c]$, $\boldsymbol{r}_{2,\lambda} = [a(0.5 - x_\lambda), b(y_\lambda - 0.5), 0.75c]$, $\boldsymbol{r}_{3,\lambda} = -\boldsymbol{r}_{1,\lambda}$, $\boldsymbol{r}_{4,\lambda} = -\boldsymbol{r}_{2,\lambda}$, where $\lambda = \mathrm{Y1}, \mathrm{Y2}$, $a$=1.0074 nm, $b$=1.1912 nm, and $c$=0.3407 nm are the lattice constants determined from the X-ray diffraction at room temperature, $x_\lambda$ and $y_\lambda$ are dimensionless atomic parameters. In particular, $x_{Y1}$=0.42312, $y_{Y1}$=0.11043, $x_{Y2}$=0.42346, $y_{Y2}$=0.61229 [S2]. The lattice constant $c$ is about three times less than $a$ and $b$, and each sublattice can be considered as an array of linear chains running along the $c$-axis (see Fig. S1a). Dysprosium ions substituting for $Y^{3+}$ ions form four magnetically nonequivalent centers with the point $C_s$ symmetry at sites corresponding to the basis vectors ($\boldsymbol{r}_{1,\mathrm{Y1}}, \boldsymbol{r}_{3,\mathrm{Y1}}$), ($\boldsymbol{r}_{2,\mathrm{Y1}}, \boldsymbol{r}_{4,\mathrm{Y1}}$), ($\boldsymbol{r}_{1,\mathrm{Y2}}, \boldsymbol{r}_{3,\mathrm{Y2}}$), ($\boldsymbol{r}_{2,\mathrm{Y2}}, \boldsymbol{r}_{4,\mathrm{Y2}}$). Impurity ions at sites with the basis vectors presented in each bracket are magnetically equivalent. In the external magnetic fields parallel to the crystallographic axes, all Dy1 (Dy2) ions are magnetically equivalent. The deformed oxygen octahedra corresponding to the first coordination shell of Y1 (Y2) ions are displayed in Figs. S1b and S1c.

## Spectroscopic studies of $SrY_2O_4:Dy^{3+}$ single crystals

### *EPR spectra*

Electron paramagnetic resonance (EPR) spectra of the oriented $SrY_2O_4:Dy^{3+}$ single crystal samples were measured with the commercial continuous mode X-band (~ 9.5 GHz) EPR spectrometer. The sample was mounted to the end of a quartz rod and placed to a center of the ER4102ST rectangular cavity operating in the $TE_{102}$ mode, and static magnetic field $\mathbf{B_0}$ and the magnetic component of the microwave radiation $\mathbf{B_1}$ are perpendicular to each other ($\mathbf{B_1} \perp \mathbf{B_0}$). For precise measurements of the orientation dependencies of the EPR spectra, the motorized rotation mount was used.

Examples of the registered signals are shown in Figs. S2 and S3. An intense central EPR line arising from even Dy-isotopes has 12 satellites that originate from two odd $^{161}Dy$ and $^{163}Dy$ isotopes, each possessing the nuclear spin $I$ = 5/2. The spectra were analyzed in the framework of the Spin-Hamiltonian approach for a system with an effective spin $S$ = 1/2 [S1].

Orientation dependences of the EPR signals from Dy1 sites were studied for the magnetic fields rotated in the *ac*, *bc* and *ab* planes (see Fig. S4). The measured principal values of $g$-factors are $g_1$=1.99394, $g_2$=2.7422, $g_3$=$g_{cc}$=13.6108, the angle between the $a$-axis and the principal $g_1$-axis equals $\theta_a(g_1) = \pm 13.9°$.

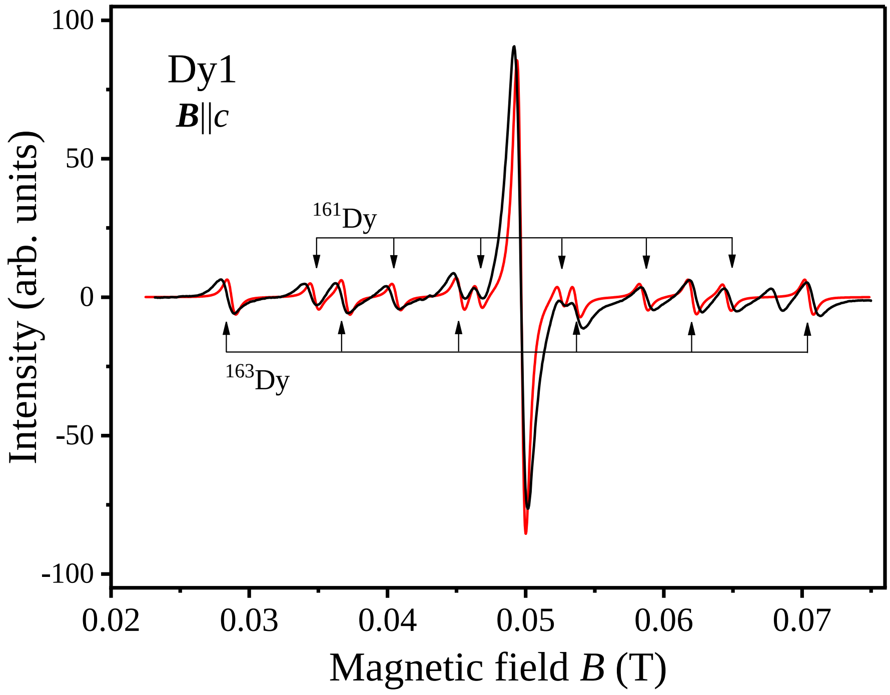


**Fig. S2.** Measured (black line) and calculated (red line) EPR signals from Dy1 ions in $SrY_2O_4:Dy^{3+}$ (0.01 at.%) single crystal, $\mathbf{B}$||$c$, frequency 9.429 GHz, $T$=10 K.

The EPR signals from Dy2 sites were registered for the magnetic fields rotated in the *ab* – plane. The maximum value of the *g*-factor $g_2$=19.28 was measured along the principal axes of the two magnetically nonequivalent Dy2 centers tilted from the *b*-axis by $\pm$8.9°. Qualitatively similar single-ion magnetic anisotropy at Dy1 and Dy2 sites in $SrDy_2O_4$ was predicted in [S5].

The simulated envelopes of the EPR signals for even and odd isotopes at Dy1 and Dy2 sites and angular dependencies of resonance magnetic fields for even isotopes at Dy1 sites are compared with the experimental data in Figs. S2-S4. The hyperfine coupling constants in the Hamiltonian of the hyperfine interaction projected on the space of electron-nuclear states of the ground multiplet $^6H_{15/2}$, $H_{HF}=A_J\mathbf{JI}$, used in simulations, equal $A_J(^{163}Dy)$ = 154.9 MHz, $A_J(^{161}Dy)$ = −110.5 MHz.

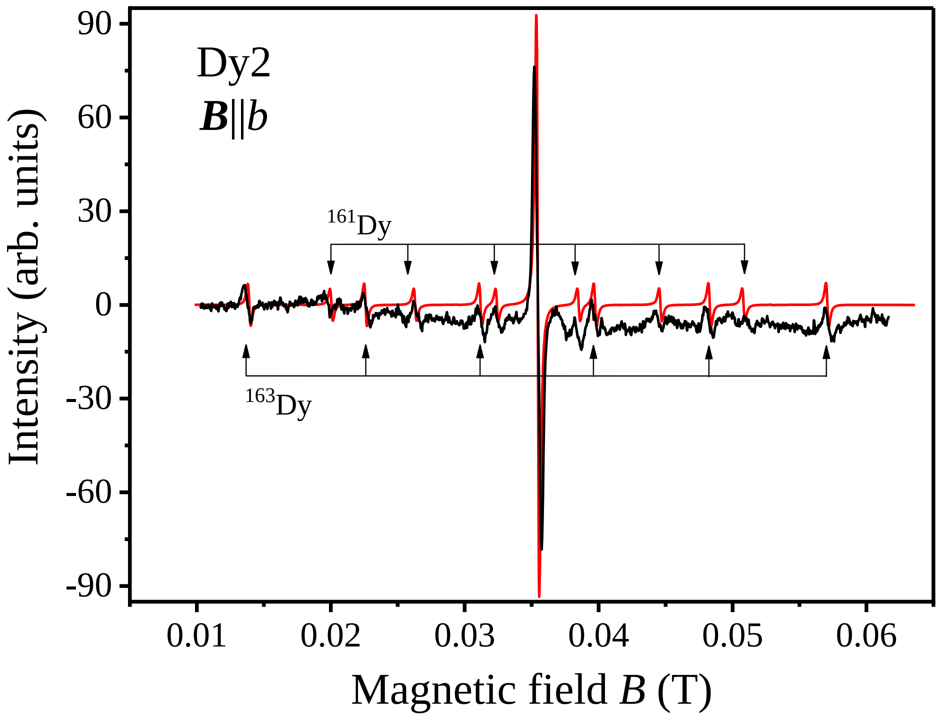


**Fig. S3.** Measured (black line) and calculated (red line) EPR signals from Dy2 centers in $SrY_2O_4:Dy^{3+}$ (0.01 at.%) single crystal, ***B***||*b*, frequency 9.433 GHz. *T*=10 K.

In the present work, the crystal-field (CF) approach to spectral properties of impurity $Dy^{3+}$ ions in $SrY_2O_4$ is derived (see below). Based on the calculations of CF parameters in the framework of the Exchange Charge Model (ECM) [S6], this approach allowed us to assign the measured EPR spectra of structurally nonequivalent paramagnetic centers (as well as the optical spectra, see below) to exact positions of $Dy^{3+}$ ions at Y1 or Y2 sites. The calculated *g*-factors of the ground state doublets of Dy1 and Dy2 ions in Table S1 agree satisfactorily with the measured EPR spectra.

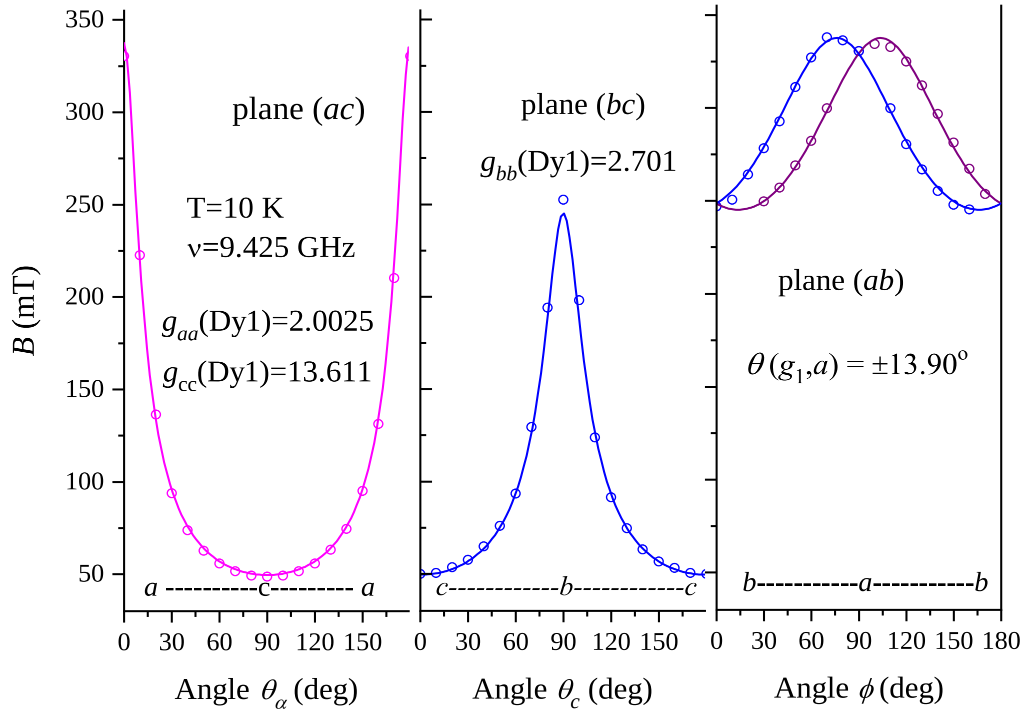


**Fig. S4.** Measured (symbols) and calculated (solid lines) angular dependencies of resonant magnetic fields for $Dy^{3+}$ ions (even isotopes) at Y1 sites.

**Table S1.** Calculated in the framework of the CF approach and measured (in brackets) principal values of $g$-tensors and directional cosines of the corresponding principal axes in the crystallographic frame for the ground state of the $Dy^{3+}$ ions substituting for Y1 (Dy1) and Y2 (Dy2) sites. The effective Lande factors are $g_J = 0.9925 \cdot 4/3$ (Dy1) and $g_J = 0.985 \cdot 4/3$ (Dy2).

| Dy1 | | | Dy2 | | |
|---|---|---|---|---|---|
| $g$-factors | cos $\theta_a$ | cos $\theta_b$ | $g$-factors | cos $\theta_a$ | cos $\theta_b$ |
| $g_1$=1.8964 (1.994) | 0.9395 | -0.3420 | $g_1$=0.0459 - | 0.9845 | -0.1753 |
| $g_2$=2.9127 (2.742) | 0.3420 | 0.9397 | $g_2$=19.2614 (19.28) | 0.1753 | 0.9845 |
| $g_3$=13.5364 (13.611) | | | $g_3$=0.0729 - | | |
| $g_{xx}$=2.042 (2.002) | | | $g_{xx}$=3.376 (~3) | | |
| $g_{yy}$=2.813 (2.701) | | | $g_{yy}$=18.963 (~19) | | |
| $\theta_a(g_1)=19.03^0$ (13.9°) | | | $\theta_b(g_2)=10.1^0$ (8.87°) | | |

***Site-selective laser spectroscopy***

Fluorescence of the crystals was excited with a pulsed tunable dye laser (Coumarin-102) pumped by the second or third harmonic of the Nd-YAG laser (LQ129, Solar LS). The linewidth of laser emission was about 0.05 nm. The spectra were analyzed with the MDR-23 monochromator. The fluorescence signal was detected by a cooled photomultiplier (FEU-106 or

FEU-83) in the photon-counting regime. The samples were placed in a bath helium cryostat and kept in the helium vapor at a temperature of 4.2 K.

Luminescence spectra corresponding to zero-phonon transitions from the lowest sublevels of the $^4F_{9/2}$ multiplet with energies $E_0$=20919 cm$^{-1}$ (Dy1) and $E_0$=21042 cm$^{-1}$ (Dy2) to CF sublevels of lower multiplets $^6H_J$ ($J$=5/2, 7/2, 9/2, 11/2, 13/2, 15/2) and $^6F_J$ ($J$=11/2, 9/2) of the two nonequivalent $Dy^{3+}$ centers in the $SrY_2O_4$:Dy (0.5 at.%) single crystal were selectively registered using the resonant laser excitation of the $Dy^{3+}$ ions to excited Stark sublevels of the $^4F_{9/2}$ multiplet. As an example, Fig. S5 shows the spectra which reveal Stark structures of the ground multiplet $^6H_{15/2}$ of Dy1 and Dy2 centers under the excitation by the laser radiation with the wavenumbers of 20941 cm$^{-1}$ and 21144 cm$^{-1}$. These resonant frequencies correspond to transitions from the ground state to the first (Dy1 centers) and the second (Dy2 centers) excited Stark sublevel of the $^4F_{9/2}$ multiplet, respectively. Lables Γ of spectral lines $^4F_{9/2}(E_0)\rightarrow{}^6H_{15/2}(\Gamma)$ in Fig. S5 correspond to notations of CF energy levels of the ground multiplet $^6H_{15/2}$ in Table S2. We note that it was not possible to resolve spectral lines corresponding to transitions which involved strongly broadened higher sublevels of multiplets. Intensities of these transitions are weaker than intensities of broad electron-vibrational bands.

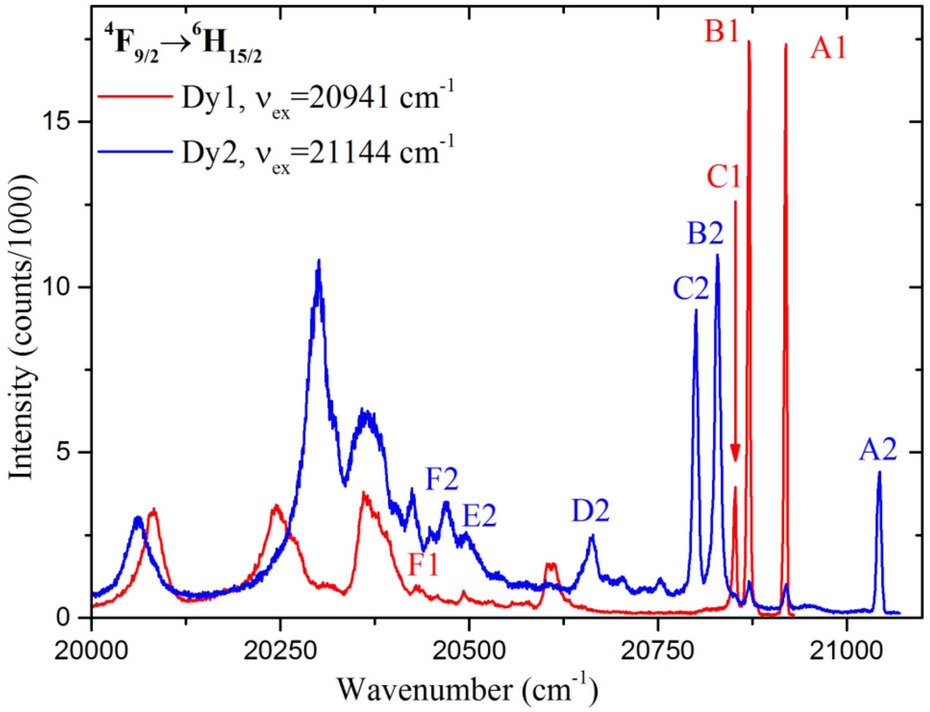


**Fig. S5.** Luminescence spectra corresponding to the emission from the lowest sublevel of the $^4F_{9/2}$ multiplet to the sublevels of the ground $^6H_{15/2}$ multiplet in Dy1 and Dy2 centers.

**Crystal field parameters for Dy1 and Dy2 centers**

Patterns of the CF energies of the Dy1 and Dy2 centers constructed on the basis of the optical

measurements (in particular, lower fragments of these patterns are presented in Table S2) were analyzed using numerical diagonalization of the Hamiltonian $H_\lambda = H_{FI} + H_{CF,\lambda}$ ($\lambda$=Dy1, Dy2) operating in the total space of states of the electronic $4f^9$ configuration of a $Dy^{3+}$ ion. Here $H_{FI}$ is the free ion standard Hamiltonian [S7] and $H_{CF,\lambda}$ is the CF interaction determined by a set of 15 CF parameters $B^k_{p,\lambda}$. In the Cartesian crystallographic frame ($x||a$, $y||b$, $z||c$)

$$\begin{aligned} H_{CF,\lambda} &= B^0_{2,\lambda}O^0_2 + B^2_{2,\lambda}O^2_2 + B^{-2}_{2,\lambda}O^{-2}_2 + B^0_{4,\lambda}O^0_4 + B^2_{4,\lambda}O^0_4 \\ &+ B^{-2}_{4,\lambda}O^{-2}_4 + B^4_{4,\lambda}O^4_4 + B^{-4}_{4,\lambda}O^{-4}_4 + B^0_{6,\lambda}O^0_6 + B^2_{6,\lambda}O^2_6 \\ &+ B^{-2}_{6,\lambda}O^{-2}_6 + B^4_{6,\lambda}O^4_6 + B^{-4}_{6,\lambda}O^{-4}_6 + B^6_{6,\lambda}O^6_6 + B^{-6}_{6,\lambda}O^{-6}_6 \end{aligned} \tag{S1}$$

where $O^k_p$ are linear combinations of spherical tensor operators which correspond to the Stevens operators in the space of eigenfunctions of an angular momentum.

The initial values of CF parameters were calculated using the ECM expressions which contain the explicit analytical dependencies of point ionic and exchange charges contributions into CF parameters for an impurity ion on coordinates of ligand and distant host crystal lattice ions $\mathbf{R}(n_1n_2n_3\kappa) = \mathbf{R}_{\kappa L} = n_1\mathbf{a} + n_2\mathbf{b} + n_3\mathbf{c} + \mathbf{r}_\kappa$ (integer numbers $n_i$ define the unit cell and $\mathbf{r}_\kappa$ is the sublattice basis vector). In the framework of the simplest ECM version, there are only two model parameters, $q_{eff}$ and $G$, that determine effective ion and exchange charges, respectively.

$$B^k_p = e^2 K^k_p \sum_{\kappa L} [\text{-}q_{eff} Z_\kappa (1\text{-}\sigma_p) \frac{<r^p>}{R^{p+1}_{\kappa L}} + \frac{2(2p+1)G}{7R_{\kappa L}} S_p(R_{\kappa L})] O^k_p(\vartheta_{\kappa L}, \varphi_{\kappa L})] \tag{S2}$$

where $e$ is the elementary charge, $K^k_p$ are the numerical factors [S6], $Z_\kappa$ is the nominal ion charge, $\sigma_p$ are the Sternhaimer shielding factors, $<r^p>$ are moments of the $4f$ electron radial wave function, $R_{\kappa L}$, $\vartheta_{\kappa L}$, $\varphi_{\kappa L}$ are spherical coordinates of host ions, $O^k_p(\vartheta, \varphi)$ are linear combinations of spherical functions corresponding to Stevens operators, and

$$S_p(R) = S^2_s(R) + S^2_\sigma(R) + \gamma_p S^2_\pi(R), \tag{S3}$$

$S_s = <4f0|n''s0>$, $S_\sigma = <4f0|n''p0>$, $S_\pi = <4f1|n''p1>$ are overlap integrals of the $4f$ wave functions with the wave functions of electrons localized on the outer closed *n’’s* and *n’’p* shells of a ligand ion at a distance $R$ from the rare-earth ion, $\gamma_2 = 3/2$, $\gamma_4 = 1/3$, $\gamma_6 = -3/2$. For $Dy^{3+}$ ions, $\sigma_2$ = 0.646, $\sigma_4 = \sigma_6 = 0$, [S8], $<r^2>=0.726$, $<r^4>=1.322$, $<r^6>=5.107$ (atomic units) [S9], the calculated overlap integrals for the $Dy^{3+}$ and $O^{2-}$ wave functions are approximated by the expressions $S_\alpha = a_\alpha \exp(-b_\alpha R^{c_\alpha})$, $a_s$=0.26533, $a_\sigma$=0.070386, $a_\pi$=1.40205, $b_s$=0.859, $b_\sigma$=0.2495, $b_\pi$=2.2761, $c_s$=1.5476, $c_\sigma$=2.2061, $c_\pi$=0.9356 (the radial wave functions were taken from [S9] and [S10] for $Dy^{3+}$ and $O^{2-}$ ions, respectively).

**Table S2**. Crystal-field energies ($cm^{-1}$) of the ground multiplet sublevels of $Dy^{3+}$ ions at Dy1 and Dy2 sites obtained from optical spectra in the present work and from inelastic neutron scattering spectra of $SrDy_2O_4$ [S11] (in brackets).

| Dy1 | | | | Dy2 | | | |
|---|---|---|---|---|---|---|---|
| | Experiment | | Theory | | Experiment | | Theory |
| A1 | 0 | | 0 | A2 | 0 | | 0 |
| B1 | 48.6 | (34.3) | 51.5 | B2 | 214.3 | (216) | 212.6 |
| C1 | 67.1 | (64) | 68.8 | C2 | 243.3 | (240) | 246.6 |
| D1 | - | (328) | 287 | D2 | 381 | (384) | 369.4 |
| E1 | - | (464) | 466 | E2 | 546 | | 538.7 |
| F1 | 486 | (488) | 485 | F2 | 620 | | 616.7 |
| G1 | - | | 585 | G2 | - | | 670.7 |
| H1 | - | | 707 | H2 | - | | 867.4 |

The ECM parameters $q_{\mathrm{eff}}$ = 0.85, $G$(Dy1)=7 and $G$(Dy2)=6.5 were determined from a comparison of the calculated and measured total splitting of the electronic multiplets $^6H_{13/2}$ and $^6H_{11/2}$, next, the calculated CF parameters were varied to fit simultaneously the measured Stark structures of all registered multiplets and the $g$-factors of the ground doublet. The final sets of CF parameters for Dy1 and Dy2 centers are presented in Table S3. The CF parameters $B^k_{p,\lambda}$ ($k$<0) for the magnetically non-equivalent sites $\mathbf{r}_{1,\lambda}$, $\mathbf{r}_{3,\lambda}$ and $\mathbf{r}_{2,\lambda}$, $\mathbf{r}_{4,\lambda}$ have the same absolute values but differ in sign.

**Table S3.** Crystal-field parameters $B^k_{p,\lambda}$ ($cm^{-1}$) for rare-earth ions in the sublattices $\mathbf{r}_{1,Y1}$, $\mathbf{r}_{3,Y1}$ and $\mathbf{r}_{1,Y2}$, $\mathbf{r}_{3,Y2}$.

| $p$ | $k$ | Dy1 | Ho1 [S2] | Er1 [S1] | Dy2 | Ho2 [S2] | Er2 [S1] |
|---|---|---|---|---|---|---|---|
| 2 | 0 | 181.5 | 200.3 | 188 | -5 | -8 | 17 |
| 2 | 2 | 90.2 | 143.1 | 137.5 | -729 | -748 | -744 |
| 2 | -2 | -113.7 | -142.6 | -171.2 | -145 | -133 | -125 |
| 4 | 0 | -64.2 | -59.45 | -57.3 | -64.7 | -63 | -60.2 |
| 4 | 2 | -1074 | -1068.3 | -1066.2 | 1103.2 | 1100 | 1033.2 |
| 4 | -2 | 1180 | 1186.6 | 1165.2 | -927.8 | -981 | -977.8 |
| 4 | 4 | -78.7 | -62.4 | -86.9 | 380.2 | 408 | 430.2 |
| 4 | -4 | -972.5 | -942 | -972.3 | -770.6 | -715 | -685.6 |
| 6 | 0 | -41.7 | -40.95 | -38 | -37.2 | -36.9 | -35.2 |
| 6 | 2 | -40 | -22.1 | -22.3 | -71.4 | -70 | -68.4 |
| 6 | -2 | 43.3 | 23.1 | 22.8 | -37.8 | -37.4 | -42.8 |
| 6 | 4 | 24.7 | 3.8 | 30.1 | -80.2 | -73 | -80.2 |
| 6 | -4 | -141.9 | -151.1 | -115.2 | -211.4 | -208 | -191.4 |
| 6 | 6 | -170.3 | -155.7 | -162.2 | -119.6 | -115 | -119.6 |
| 6 | -6 | -89.25 | -99.3 | -84 | 90.5 | 95 | 80.5 |

The calculated $g$-factors of the ground doublets and CF energies of sublevels of the ground multiplet are compared with the measured values in Tables S1 and S2. A near-monotonous

variation of CF parameters along the lanthanide series (see Table S3) and achieved over-all agreement between the calculated and measured spectral parameters evidences for reasonable results of the crystal-field modeling and the identification of the observed spectral lines with zero-phonon transitions in the Dy1 and Dy2 centers.

**Parameters of electron-phonon interaction**

The electronic operators $V_{\alpha\beta} = \sum_{pk} b^k_{p,\alpha\beta} O^k_p$ in the Hamiltonian of the electron-phonon interaction are linear combinations of Stevens operators $O^k_p$ with coefficients (EPI parameters)

$$b^k_{p,\alpha\beta} = \frac{1}{2}\sum_{L\kappa}\left(\frac{\partial B^k_p(\{\mathbf{R}\})}{\partial R_{\kappa L,\beta}} + \frac{\partial B^k_p(\{\mathbf{R}\})}{\partial R_{\kappa L,\alpha}}\right). \quad \text{(S4)}$$

Here the sum is taken over lattice ions with the radius-vectors $\mathbf{R}_{\kappa L}$ in the crystallographic system of coordinates with the origin on the considered rare-earth ion. The calculated sets of EPI parameters within the framework of the exchange charge model with the same model parameters as in the calculations of the CF parameters are presented in Tables S4 and S5.

**Table S4.** Parameters of the electron-phonon interaction $b^k_{p,\alpha\beta,1}$ (cm$^{-1}$) for Dy1 sites $\mathbf{r}_{1,Y1}$.

| $p$ $k$ | $b^k_{p,xx,1}$ | $b^k_{p,yy,1}$ | $b^k_{p,zz,1}$ | $b^k_{p,xy,1}$ | $p$ $k$ | $b^k_{p,xz,1}$ | $b^k_{p,yz,1}$ |
|---|---|---|---|---|---|---|---|
| 2 0 | 1013 | -1114 | 2.4 | -2490 | 2 1 | 1059 | -6527 |
| 2 2 | -387.9 | -37.5 | 319.2 | 4441 | 2 -1 | -4904 | -7083 |
| 2 -2 | 2443 | -1998 | -400.2 | -782.5 | 4 1 | -1680 | -844.2 |
| 4 0 | -112.4 | 104.5 | 75.8 | 237.0 | 4 -1 | -844.9 | -3048 |
| 4 2 | 588.6 | 167.4 | 427.2 | 473.9 | 4 3 | 3033 | 11260 |
| 4 -2 | -189.2 | -663.4 | -491.0 | 230.7 | 4 -3 | 2402 | 1911 |
| 4 4 | 543.6 | -496.6 | 30.9 | 522.9 | 6 1 | 550.5 | 206.4 |
| 4 -4 | 1285 | -442.0 | 356.9 | -2115 | 6 -1 | 206.4 | 971.4 |
| 6 0 | 12.2 | 29.1 | 11.0 | 23.2 | 6 3 | 507.0 | 2890 |
| 6 2 | -191.3 | 219.0 | -22.7 | 850.6 | 6 -3 | 2545 | 258.7 |
| 6 -2 | 403.0 | -447.5 | 15.3 | -644.1 | 6 5 | -2610 | -1082 |
| 6 4 | -417.2 | 416.1 | 23.8 | -703.7 | 6 -5 | -3000 | 2323 |
| 6 -4 | -280.0 | 296.4 | 192.4 | 747.4 | | | |
| 6 6 | 678.9 | -429.1 | 20.5 | -125.7 | | | |
| 6 -6 | -381.6 | 573.6 | 13.6 | -1105 | | | |

**Table S5.** Parameters of the electron-phonon interaction $b^k_{p,\alpha\beta,2}$ (cm$^{-1}$) for Dy2 sites $\mathbf{r}_{1,Y2}$..

| $p$ $k$ | $b^k_{p,xx,2}$ | $b^k_{p,yy,2}$ | $b^k_{p,zz,2}$ | $b^k_{p,xy,2}$ | $p$ $k$ | $b^k_{p,xz,2}$ | $b^k_{p,yz,2}$ |
|---|---|---|---|---|---|---|---|
| 2 0 | -1186 | 1162 | 79.3 | 1704.5 | 2 1 | -6600 | 4719 |
| 2 2 | -710.5 | 1388 | -248.4 | 2808 | 2 -1 | 3488 | 3554 |
| 2 -2 | 1283 | 1527 | 303.7 | 863.1 | 4 1 | -2054 | 522.4 |
| 4 0 | 139.2 | -147.6 | 62.7 | -168.0 | 4 -1 | 522.4 | -1726 |
| 4 2 | -49.9 | -757.2 | -380.0 | 593.0 | 4 3 | -2371 | 4842 |
| 4 -2 | 592.0 | -1.0 | 338.9 | -115.0 | 4 -3 | 6403 | -3381 |
| 4 4 | 493.4 | -838.0 | -77.4 | 54.1 | 6 1 | 1007 | -318.4 |
| 4 -4 | -77.3 | 583.2 | 225.2 | -46.7 | 6 -1 | -318.4 | 679.0 |
| 6 0 | 19.3 | 16.7 | 6.5 | -28.6 | 6 3 | -291.7 | 1595 |
| 6 2 | -310.6 | 347.3 | 48.9 | 509.3 | 6 -3 | 2156 | 557.6 |
| 6 -2 | 275.2 | -234.1 | -29.2 | -318.4 | 6 5 | 1542 | 1822 |
| 6 4 | 134.1 | -51.7 | 14.4 | 46.3 | 6 -5 | 1145 | -535.5 |
| 6 -4 | 223.4 | -145.2 | 157.4 | -222.0 | | | |
| 6 6 | 46.0 | 8.0 | 31.7 | -143.9 | | | |
| 6 -6 | -147.3 | 69.2 | 5.6 | -85.6 | | | |

## Cross-relaxation

In the case of the local $C_s$ symmetry, the CR transition probabilities (14) contain 13 nonzero lattice sums $k^{\lambda\lambda'}_{\alpha\beta,\gamma\delta}$ for fixed sublattices $\lambda$ and $\lambda'$. The computed lattice sums in Voight notations equal (in the units of $10^3$/nm$^6$)

for magnetically equivalent ions $\lambda = \lambda' = \text{Dy2}$

$k_{11}$ = 1.572; $k_{22}$ = 1.852; $k_{33}$ = 5.318;
$k_{44}$ = 1.348; $k_{55}$ = 0.548; $k_{66}$ = 1.277;
$k_{12}$ = 0.947; $k_{13}$ = -2.519; $k_{16}$ = 0.4217;
$k_{23}$ = -2.799; $k_{26}$ = -0.707; $k_{36}$ = 0.2854; $k_{45}$ = -0.761;

for $\lambda = \lambda' = \text{Dy1}$

$k_{11}$ = 1.610; $k_{22}$ = 1.908; $k_{33}$ = 5.317;
$k_{44}$ = 1.463; $k_{55}$ = 0.5574; $k_{66}$ = 1.289;
$k_{12}$ = 0.8995; $k_{13}$ = -2.510; $k_{16}$ = 0.4719;
$k_{23}$ = -2.807; $k_{26}$ = -0.754; $k_{36}$ = 0.2822; $k_{45}$ = -0.8034;

and for magnetically nonequivalent ions $\lambda = \text{Dy2}$, for $\lambda' = \text{Dy1}$

$k_{11}$ = 1.677; $k_{22}$ = 1.437; $k_{33}$ = 0.448;
$k_{44}$ = 0.678; $k_{55}$ = 1.154; $k_{66}$ = 0.582;
$k_{12}$ = -1.333; $k_{13}$ = -0.344; $k_{16}$ = -0.2474;
$k_{23}$ = -0.1042; $k_{26}$ = 0.4355; $k_{36}$ = -0.188; $k_{45}$ = 0.2625.

**Hysteresis loops**

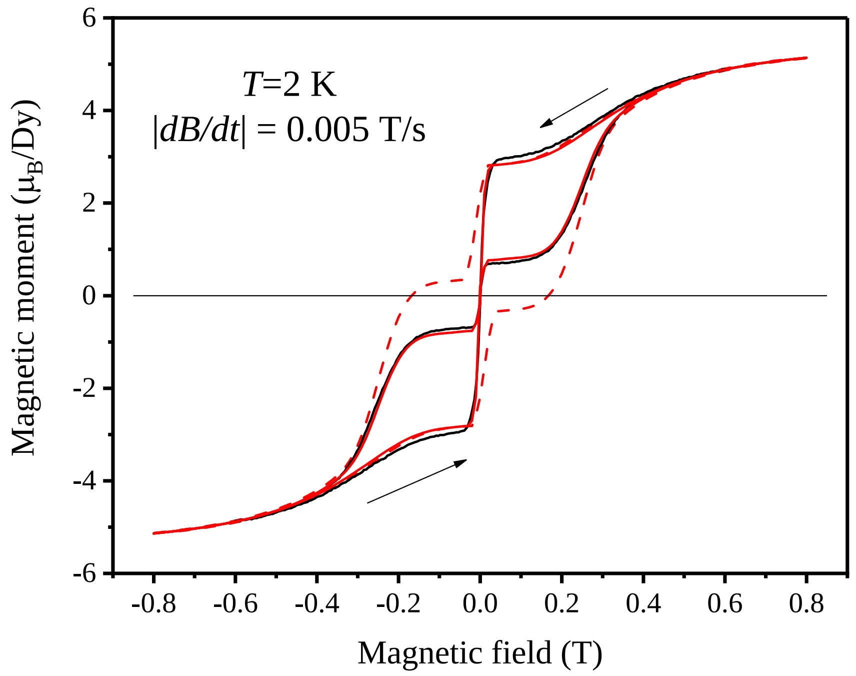


**Fig. S6.** Computed dynamic magnetization of the $SrY_2O_4$:Dy (0.01 at%) single crystal with (red solid lines) and without (dash red lines) accounting for the cross-relaxation in comparison to the measured double-loop hysteresis (black lines).

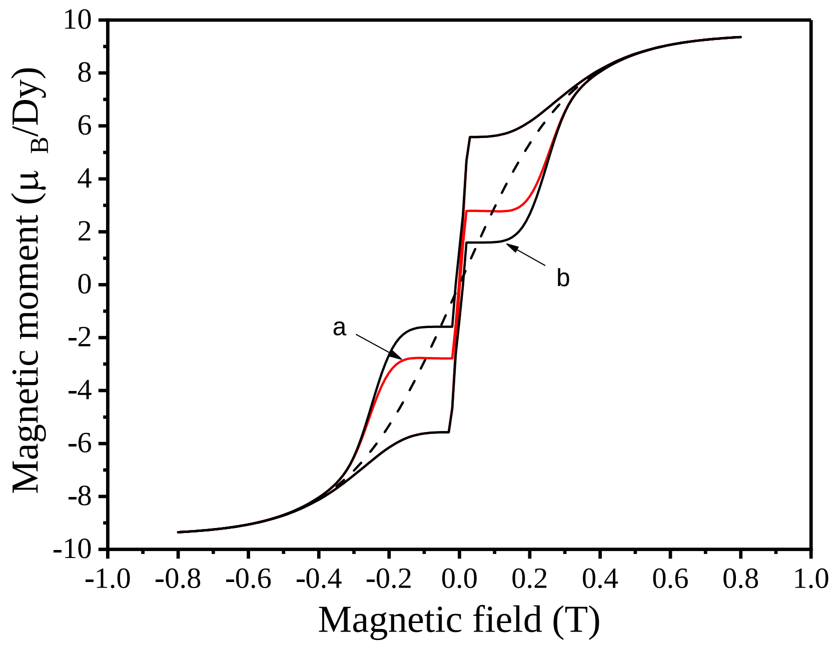


**Fig. S7.** Computed dynamic magnetization of $^{163}$Dy2 ions (a) with and (b) without accounting for the quadrupole hyperfine interaction. |*dB/dt*|=0.005 T/s, *T*=2 K. Computed equilibrium magnetization is presented by a dash line.

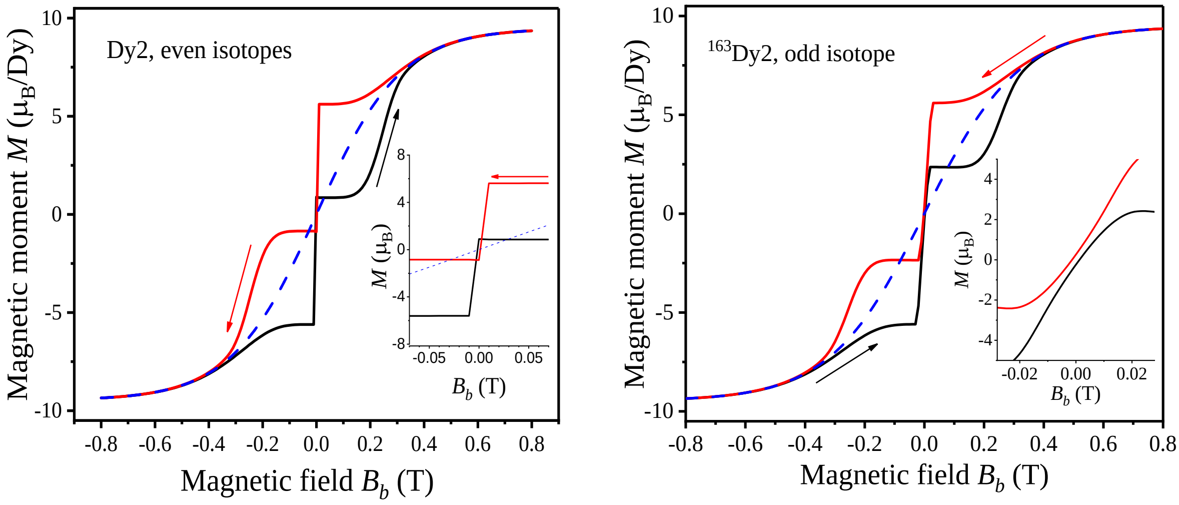


**Fig. S8.** Computed dynamic magnetization of different Dy isotopes at sites Y2 in $SrY_2O_4$:Dy (0.01 at.%), $T$=2 K , $|dB_b/dt|$ = 0.005 T/s. Dash lines show the equilibrium isothermal magnetization. The regions nearby the zero value of the swept field are in insets.

## References

[S1] B. Z. Malkin, S. I. Nikitin, I. E. Mumdzhi, D. G. Zverev, R. V. Yusupov, I. F. Gilmutdinov, R. Batulin, B. F. Gabbasov, A. G. Kiiamov, D. T. Adroja, O. Young, O. A. Petrenko, Magnetic and spectral properties of the multisublattice oxides $SrY_2O_4:Er^{3+}$ and $SrEr_2O_4$, Phys. Rev. B **92**, 094415 (2015). DOI: 10.1103/PhysRevB.92.094415.

[S2] S. I. Nikitin, E. M. Kutasheva, R. V. Yusupov, R. G. Batullin, A. G. Kiiamov, I. E. Mumdzhi, B. Z. Malkin, Site-selective laser spectroscopy of impurity $Ho^{3+}$ ions in $SrY_2O_4$ single crystals, Optics and Spectroscopy, **131**, 441 (2023). DOI: 10.21883/OS.2023.04.55546.77-22.

[S3] H. Muller-Buschbaum, Zur Kenntnis von $SrY_2O_4$, Z. Anorg. Allg. Chem. **358**, 138 (1968). DOI: 10.1002/zaac.19683580305.

[S4] Gladys H. Fuller, Nuclear spins and moments, J. Phys. Chem. Ref. Data **5**, 835 (1976).

[S5] A. Fennell, V. Y. Pomjakushin, A. Uldry, B. Delley, B. Prevost, A. Desilets-Benoit, A. D. Bianchi, R. I. Bewley, B. R. Hansen, T. Klimczuk, R. J. Cava, and M. Kenzelmann, Evidence for $SrHo_2O_4$ and $SrDy_2O_4$ as model $J_1$- $J_2$ zigzag chain materials, Phys. Rev. B **89**, 224511 (2014). DOI: 10.1103/PhysRevB.89.224511.

[S6] B. Z. Malkin, Crystal field and Electron–Phonon Interaction in Rare-Earth Ionic Paramagnets, in: Spectroscopy of solids containing rare-earth ions, ed. by A. A. Kaplyanskii and R. M. Macfarlane, Elsevier Science Publishers, Amsterdam, 1987, ch. 2, p. 13-49. DOI: 10.1016/B978-0-444-87051-3.50008-0.

[S7] W. T. Carnall, G. L. Goodman, K. Rajnak, and R. S. Rana, A systematic analysis of the spectra of the lanthanides doped into single crystal $LaF_3$, J. Chem. Phys. **90,** 3443 (1989). DOI: 10.1063/1.455853.

[S8] P. Erdos and J.H. Kang, Electronic Shielding of $Pr^{3+}$ and $Tm^{3+}$ Ions in Crystals, Phys. Rev. B **6**, 3393 (1972). DOI:10.1103/PhysRevB.6.3393.

[S9] A. J. Freeman and R. E. Watson, Theoretical Investigation of Some Magnetic and Spectroscopic Properties of Rare-Earth Ions, Phys. Rev. **127**, 2058 (1962).
DOI: 10.1103/PhysRev.127.2058.

[S10] E. Clementi and A.D. McLean, Atomic Negative Ions, Phys. Rev. A **133**, 419 (1964). DOI:10.1103/PhysRev.133.A419.

[S11] N. Gauthier, A. Fennell, B. Prévost, A.-C. Uldry, B. Delley, R. Sibille, A. Désilets-Benoit, H. A. Dabkowska, G. J. Nilsen, L.-P. Regnault, J. S. White, C. Niedermayer, V. Pomjakushin, A. D. Bianchi, and M. Kenzelmann, Absence of long-range order in the frustrated magnet $SrDy_2O_4$ due to trapped defects from a dimensionality crossover, Phys. Rev. B **95**, 134430 (2017).
DOI: 10.1103/PhysRevB.95.134430.
